# Supplementary material for: Imitation Learning via Off-Policy Distribution Matching
Source: arXiv:1912.05032 source file (2019-12-10)
Supplement: Supplementary file 1 [file appendix.tex]

\appendix

\section{Implementation Details}
All algorithms use networks with an MLP architecture with 2 hidden layers and 256 hidden units. For discriminators, critic, $\nu$ we use Adam optimizer with learning rate $10^{-3}$ while for the actors we use the learning rate of $10^{-5}$.
For the discriminator and $\nu$
networks we use gradient penalties from \cite{gulrajani2017improved}. We also regularize the actor network with the orthogonal regularization \citep{brock2018large} with a coefficient $10^{-4}$. Also we perform 4 updates per 1 environment step. We handle absorbing states of the environments similarly to \cite{kostrikov2018discriminatoractorcritic}.

\section{Algorithms}

In this section, we present pseudocode for the imitation learning algorithms based on DualDICE.

\begin{algorithm}[H]
    \textbf{Input}: expert replay buffer $\mathcal{R}_E$
    \caption{\ourname}
    \begin{algorithmic}
    \State Initialize replay buffer $\mathcal{R} \gets \emptyset$
    \For{$n=1,\ldots,$}
        \State Sample $(s, a, s')$ with $\pi_\theta$
        \State Add $(s, a, s')$ to the replay buffer $\mathcal{R}$
        \State $\{(s^{(i)} ,a^{(i)}, s^{\prime (i)})\}_{i=1}^B \sim \mathcal{R}$
        \Comment Geometric sampling
        \State $\{(s_0^{(i)}, s_E^{(i)},a_E^{(i)}, s_{E}^{\prime (i)})\}_{i=1}^B \sim \mathcal{R}_E$
        \Comment Geometric sampling, $s_0^{(i)}$ is a starting episode state for $s_E^{(i)}$
        \State $a_{0}^{(i)} \sim \pi_\theta(\cdot | s_{0}^{(i)})$, for $i=1, \ldots, B$
        \State $a^{\prime (i)} \sim \pi_\theta(\cdot | s^{\prime(i)})$, for $i=1, \ldots, B$
        \State $a_E^{\prime (i)} \sim \pi_\theta(\cdot | s_E^{\prime(i)})$, for $i=1, \ldots, B$
        \State Compute loss on expert data:
        \State $\hat{J}_{log} = \log( \frac{1}{B}\sum_{i=1}^B  ((1 - \alpha) e^{\nu_{\psi}(s_E^{(i)}, a_E^{(i)}) - \gamma \nu_{\psi}(s_E^{\prime (i)}, a_E^{\prime (i)})} + \alpha e^{\nu_{\psi}(s^{(i)}, a^{(i)}) - \gamma \nu_{\psi}(s^{\prime (i)}, a^{\prime (i)})} ) )$
        \State Compute loss on the replay buffer:
        \State $\hat{J}_{linear} = \frac{1}{B} \sum_{i=1}^B ((1 - \alpha)  (1 - \gamma) \nu_{\psi}(s_{0}^{(i)}, a_{0}^{(i)}) +  \alpha (\nu_{\psi}(s^{(i)}, a^{(i)}) -\gamma \nu_{\psi}(s^{\prime (i)}, a^{\prime (i)})))$
        \State Update $\psi \leftarrow \psi - \eta_{\nu} \nabla_{\psi} (\hat{J}_{log} - \hat{J}_{linear})$
        \State Update $\theta \leftarrow \psi + \eta_{\pi} \nabla_{\theta} (\hat{J}_{log} - \hat{J}_{linear})$
    \EndFor
    \end{algorithmic}
    \label{algo:ours}
\end{algorithm}

\comment{
\begin{algorithm}[H]
    \textbf{Input}: expert replay buffer $\mathcal{R}_E$
    \caption{\othername}
    \begin{algorithmic}
    \State Initialize replay buffer $\mathcal{R} \gets \emptyset$
    \For{$n=1,\ldots,$}
        \State Sample $(s, a, s')$ with $\pi_\theta$
        \State Add $(s, a, s')$ to the replay buffer $\mathcal{R}$
        \State $\{(s^{(i)} ,a^{(i)}, s^{\prime (i)})\}_{i=1}^B \sim \mathcal{R}$
        \Comment Geometric sampling
        \State $\{(s_0^{(i)}, s_E^{(i)},a_E^{(i)}, s_{E}^{\prime (i)})\}_{i=1}^B \sim \mathcal{R}_E$
        \Comment Geometric sampling, $s_0^{(i)}$ is a starting episode state for $s_E^{(i)}$
        \State $a_{0}^{(i)} \sim \pi_\theta(\cdot | s_{0}^{(i)})$, for $i=1, \ldots, B$
        \State $a^{\prime (i)} \sim \pi_\theta(\cdot | s^{\prime(i)})$, for $i=1, \ldots, B$
        \State $a_E^{\prime (i)} \sim \pi_\theta(\cdot | s_E^{\prime(i)})$, for $i=1, \ldots, B$
        \State Compute loss on expert data:
        \State $\hat{J}_{R_E} = \frac{1}{B} \sum_{i=1}^B (\nu_{\psi}(s_E^{(i)}, a_E^{(i)}) - \gamma \nu_{\psi}(s_E^{\prime (i)}, a_E^{\prime (i)})) \zeta_{\theta}(s_E^{(i)}, a_E^{(i)}) - f^*(\zeta_{\theta}(s_E^{ (i)}, a_E^{ (i)})) - (1 - \gamma) \nu_{\psi}(s_{0}^{(i)}, a_{0}^{(i)}) $
        \State Compute loss on the replay buffer:
        \State $\hat{J}_{R} = \frac{1}{B} \sum_{i=1}^B (\nu_{\psi}(s^{(i)}, a^{(i)}) - \gamma \nu_{\psi}(s^{\prime (i)}, a^{\prime (i)})) \zeta_{\theta}(s^{(i)}, a^{(i)}) - f^*(\zeta_{\theta}(s^{ (i)}, a^{ (i)})) -  (\nu_{\psi}(s^{(i)}, a^{(i)}) - \gamma  \nu_{\psi}(s^{\prime (i)}, a^{\prime (i)}))$
        \State Update $\psi \leftarrow \psi - \eta_{\nu} \nabla_{\psi} ((1 - \alpha) \hat{J}_{R_E} + \alpha\hat{J}_{R})$
        \State Update $\theta \leftarrow \theta + \eta_{\theta} \nabla_{\theta} ((1 - \alpha) \hat{J}_{R_E} + \alpha\hat{J}_{R})$
        \State Update actor, critic and temperature parameter $\nigma$ using rewards $r(s,a) = g(\zeta_\theta(s, a))$
    \EndFor
    \end{algorithmic}
    \label{algo:value_dice}
\end{algorithm}
}

\comment{
\section{Matching Occupancy in Tabular MDPs}

We illustrate the properties of \ourname on a simple tabular MDP with 8 states and 2 actions that transition between these states (see Fig. \ref{fig:deterministic}, 0 is the only starting state). First, we consider a deterministic agent that visits only 3 state (see Fig. \ref{fig:deterministic}). Due to the regularization with the samples from the replay buffer \ourname is able to recover an optimal policy for the states not see in the expert demonstrations. Then, we evaluate a KL divergence between occupancies on a stochastic expert (see Fig. \ref{fig:stochastic}). \ourname matches occupancies of the policies and accurately recovers the expert policy.

\begin{figure}
\centering
\begin{tikzpicture}
\tikzset{
 EdgeStyle/.append style = {->, bend left = 40} }
\Vertex{6}(A)
\Vertex[x=0.5, y = 1.5]{7}(B)
\Vertex[x=2, y = 2]{0}(C)
\Vertex[x=3.5, y = 1.5]{1}(D)
\Vertex[x=4, y = 0]{2}(E)
\Vertex[x=3.5, y = -1.5]{3}(F)
\Vertex[x=2, y = -2]{4}(G)
\Vertex[x=0.5, y = -1.5]{5}(H)
\Edge[label=1](0)(1)
\Edge[label=0](1)(0)
\Edge[label=1](1)(2)
\Edge[label=1](2)(1)
\Edge(2)(3)
\Edge(3)(2)
\Edge(3)(4)
\Edge(4)(3)
\Edge(4)(5)
\Edge(5)(4)
\Edge(5)(6)
\Edge(6)(5)
\Edge(6)(7)
\Edge(7)(6)
\Edge(7)(0)
\Edge[label=0](0)(7)
\end{tikzpicture}
\begin{tikzpicture}
\tikzset{
 EdgeStyle/.append style = {->, bend left = 40} }
\Vertex{6}(A)
\Vertex[x=0.5, y = 1.5]{7}(B)
\Vertex[x=2, y = 2]{0}(C)
\Vertex[x=3.5, y = 1.5]{1}(D)
\Vertex[x=4, y = 0]{2}(E)
\Vertex[x=3.5, y = -1.5]{3}(F)
\Vertex[x=2, y = -2]{4}(G)
\Vertex[x=0.5, y = -1.5]{5}(H)
\Edge[label=1](0)(1)
\Edge[label=0](0)(7)
\Edge[label=0](1)(0)
\Edge[label=1](1)(2)
\Edge[label = 0](2)(3)
\Edge[label = 1](2)(1)
\Edge[label = 0](3)(4)
\Edge[label = 1](3)(2)
\Edge[label = 1](4)(3)
\Edge[label = 0](4)(5)
\Edge[label = 1](5)(4)
\Edge[label = 0](5)(6)
\Edge[label = 0](6)(5)
\Edge[label = 1](6)(7)
\Edge[label = 0](7)(6)
\Edge[label = 1](7)(0)
\end{tikzpicture}
\caption{A tabular MDP with action probabilities. Left: deterministic expert demonstrations cover only 3 states (left). Right: a policy learned with \ourname produces an optimal policy for all states.
\label{fig:deterministic}
}
\end{figure}

\begin{figure}
\centering
\begin{tikzpicture}
\tikzset{
  EdgeStyle/.append style = {->, bend left = 40} }
\Vertex{6}(A)
\Vertex[x=0.5, y = 1.5]{7}(B)
\Vertex[x=2, y = 2]{0}(C)
\Vertex[x=3.5, y = 1.5]{1}(D)
\Vertex[x=4, y = 0]{2}(E)
\Vertex[x=3.5, y = -1.5]{3}(F)
\Vertex[x=2, y = -2]{4}(G)
\Vertex[x=0.5, y = -1.5]{5}(H)
\Edge[label=0.75](0)(1)
\Edge[label=0.25](0)(7)
\Edge[label=0.75](1)(2)
\Edge[label=0.25](1)(0)
\Edge[label = 0.25](2)(3)
\Edge[label = 0.75](2)(1)
\Edge[label = 0.25](3)(4)
\Edge[label = 0.75](3)(2)
\Edge[label = 0.25](4)(5)
\Edge[label = 0.75](4)(3)
\Edge[label = 0.25](5)(6)
\Edge[label = 0.75](5)(4)
\Edge[label = 0.25](6)(7)
\Edge[label = 0.75](6)(5)
\Edge[label = 0.25](7)(0)
\Edge[label = 0.75](7)(6)
\end{tikzpicture}
\begin{tikzpicture}
\begin{axis}[
width=0.5\textwidth,
axis lines= left,
    ymin=0,
  ylabel=KL,
  xlabel=Updates,
  ymode=log,
  xticklabel style = {rotate=30,anchor=east},
  xticklabels from table={kl_plot.tex}{X},xtick=data]
\addplot[red,thick,mark=square*] table [x=X, y=Y]{kl_plot.tex};
\end{axis}
\end{tikzpicture}
\caption{A tabular MDP with action probabilities. Left: a stochastic expert visit all states starting from state 0. Right: \ourname matches the occupancy and recover the stochastic policy.
\label{fig:stochastic}
}
\end{figure}
}

\section{Additional experiments}

We also compared \ourname with behavioral cloning in the offline regime, when we sample no additional transitions from the learning environment (see Figure \ref{fig:offline_app}). Even given only offline data, \ourname outperforms behavioral cloning. For behavioral cloning we used the same regularization as for actor training in \ourname.

\begin{figure}[h]
\centering
\includegraphics[width=0.2\textwidth]{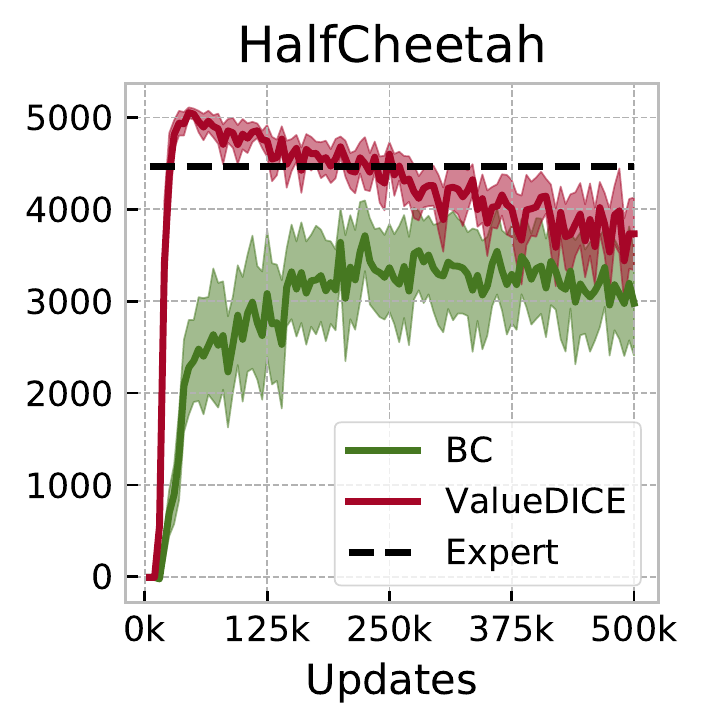}
\includegraphics[width=0.2\textwidth]{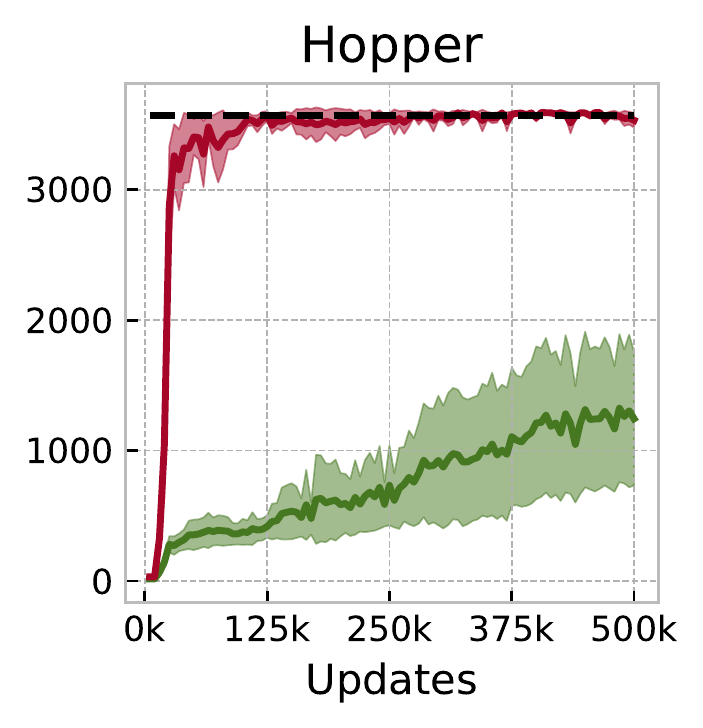} 
\includegraphics[width=0.2\textwidth]{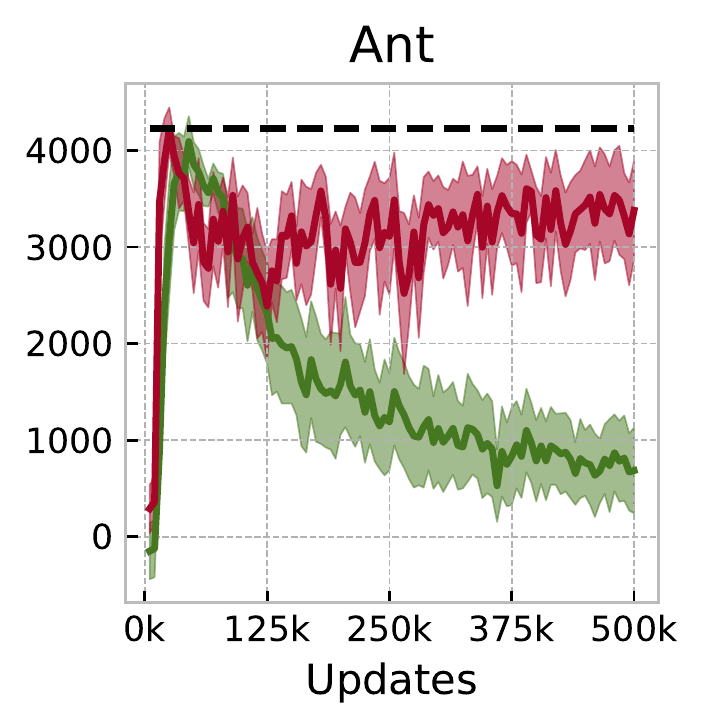}
\includegraphics[width=0.2\textwidth]{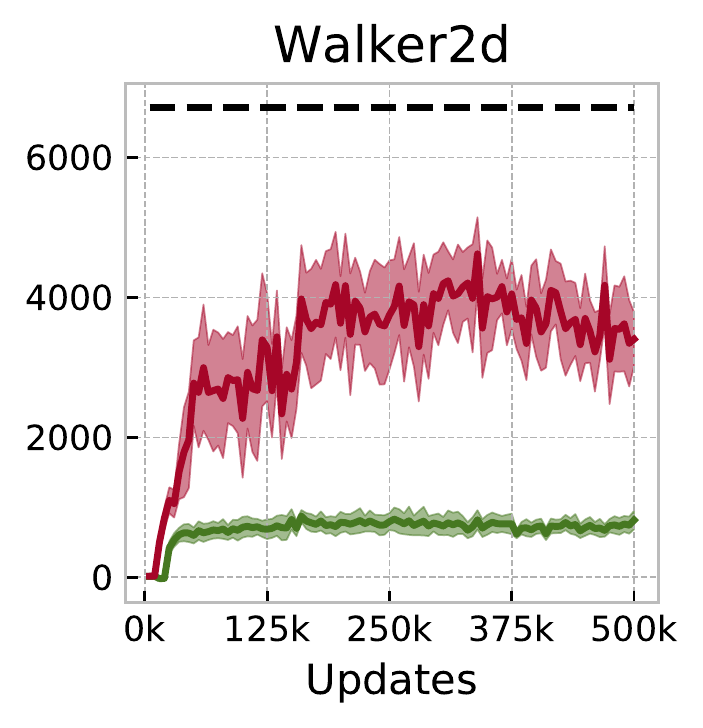}
\caption{\ourname outperforms behavioral cloning given 1 trajectory even without replay regularization.}
\label{fig:offline_app}
\end{figure}

\comment{
\section{Comparison with \othername}

As we mention in section \ref{sec:offdualdice}, rewards obtain from \othername can be used in a combination with an off-policy RL algorithm. In this section, we compare \othername with \ourname that learns a value function directly without extracting these rewards. We use SAC specifically with the same hyper parameters as in Section \ref{sec:experiments}. To learn the rewards we use a duality discussed in \citep{nachum2019dualdice}. For \othername we use Adam optimizer with learning rates $10^{-4}$ and $10^-3$ for $\nu$ and $\zeta$ respectively. We regularize both $\nu$ and $\zeta$ with gradient penalty \citep{gulrajani2017improved}. Also for \othername we use a different representation of KL:
\begin{equation}
\label{eq:kl-donsker}
-\dkl\left(\dpi || \dexpert \right) =  \inf_{x: \S \times \A \to \R} \E_{(s, a) \sim \dexpert} [ e^{x(s, a)}] - \E_{(s, a) \sim \dpi}  [x(s, a)].
\end{equation}

Thus, for the experiments, we used $f^*(x) = x \log(x) - x$ and $g(x)=x$.

\begin{figure}
\centering
\includegraphics[width=0.24\textwidth]{imgs/results_appndx/HalfCheetah_1appndx.pdf}
\includegraphics[width=0.24\textwidth]{imgs/results_appndx/Hopper_1appndx.pdf}
\includegraphics[width=0.24\textwidth]{imgs/results_appndx/Walker2d_1appndx.pdf}
\caption{Comparison of algorithms given 1 expert trajectory. \ourname demonstrates best performance on all tasks.}
\label{fig:res1}
\end{figure}

\begin{figure}
\centering
\includegraphics[width=0.24\textwidth]{imgs/results_appndx/HalfCheetah_10appndx.pdf}
\includegraphics[width=0.24\textwidth]{imgs/results_appndx/Hopper_10appndx.pdf} 
\includegraphics[width=0.24\textwidth]{imgs/results_appndx/Walker2d_10appndx.pdf}
\caption{Comparison of algorithms given 10 expert trajectories. \ourname outperforms the other method. However, given this amount of data, behavioral cloning can recover the expert policy as well.}
\label{fig:res2}
\end{figure}
}
